# Supplementary material for: On the limits of agency in agent-based models
Source: arXiv:2409.10568 source file (2024-11-10)
Supplement: Supplementary file 1 [file appendix.tex]

\newpage
\appendix

\section{Appendix A: AgentTorch framework}
\textbf{Code}: The AgentTorch project is open-source at \url{github.com/AgentTorch/AgentTorch} and the documentation is available at \url{https://agenttorch.github.io/AgentTorch/}.
Some quick links are given below -
\begin{itemize}
    \item Architecture: \url{https://agenttorch.github.io/AgentTorch/architecture/}
    \item Installation: \url{https://agenttorch.github.io/AgentTorch/install/}
    \item Contributing: \url{https://agenttorch.github.io/AgentTorch/contributing/}
    \item Getting Started: \url{https://agenttorch.github.io/AgentTorch/tutorials/creating-a-model/}
\end{itemize}
The GitHub repository includes sample models to get started and interactive tutorials to implement new models and analyze existing ones.

\begin{figure*}[h!]
    \centering
    \includegraphics[width=0.97\textwidth]{appendix_figs/diff_eg_code.png}
    \caption{AgentTorch provides custom utilities to differentiate through discrete stochastic and conditional operations. The example here contrasts the Bernoulli distribution, where using `agent\_torch.Bernoulli` can provide a gradient unlike `torch.Bernoulli`, and is compatible with `torch.tensor`. Several such distributions, like `Binomial` or `Categorical`, are implemented in AgentTorch to provide (low-bias low-variance) gradients. AgentTorch implements discrete distributions using stochastic triples, as introduced in ~\cite{arya2022automatic} and also supported in `Julia` programming language with `StochasticAD` package. These utilities help design ABMs as differentiable programs and ensures composability of ABMs with DNNs. We refer to the GitHub source for implementations for logical operators (e.g., agent\_torch.logical\_and) and comparators in AgentTorch (e.g., agent\_torch.max)}
    
    \label{fig:code-snippet-diff}
\end{figure*}

\textbf{Differentiability}: As we discussed, differentiability is a key attribute of AgentTorch models. AgentTorch uses autograd primitives to represent a ABMs with dynamics and interventions on a compute graph, which streamlines backpropagation. However, unlike DNNs on computation graphs, defining ABMs relies extensively on mechanistic operators (torch.max, torch.compare, torch.logical\_and) to describe stochastic and conditional program flows. (e.g., offer a vaccine if age < 60, COVID-19 test has 65\% specificity). However, these operators are conventionally non-differentiable in torch and can cause incompatibility with autograd. AgentTorch implements custom operators to differentiate through stochastic and conditional programs, ensuring gradient flow through the ABM. A sample code-snippet is given in figure~\ref{fig:code-snippet-diff}. To realize this, AgentTorch integrates recent advancements in differentiable programming~\cite{yin2019understanding,arya2022automatic} to provide a simple-to-use API for achieving low-bias low-variance gradients during backpropagation. We note this is important for agent-based modeling since gradient estimators that work well for neural network training (with millions of parameters and limited stochasticity) may not generalize well for simulations (with low-dim parameters and compositional stochasticity). For example, the Gumbel-Softmax reparameterization is shown to work well in variational autoencoders (VAEs) but fails with ABMs since it has a high-biased under composition~\cite{friede2021efficient}. On GitHub, we recommend looking at \url{agent_torch/distributions} and \url{agent_torch/helpers/soft.py} for differentiable implementations of discrete distributions and conditional operators.

\section{Appendix B: Environment and Agent specification}
We provide additional details about the simulation environment, data sources, system prompt, and agent specification for our case study experiment.

\textbf{Agent}:
We consider 8.4 million agents that can catch and transmit infections, and be willfully employed. Their state is composed of static (age, gender, income, occupation, household, geo-location) and dynamic attributes (disease status, employment status). The demographic and household characteristics are sampled using the 2022 American community survey (ACS), employment characteristics from the bureau of labor statistics and disease dynamics from the CDC. Agents interact with each other over household, workplace, and mobility networks. We parameterize interactions for recreational and workplace mobility using Google Mobility trends; and household interactions are obtained from the ACS household and migration survey. The census provides summary statistics, which we use to initialize the synthetic populations using standard methods like iterative proportional fitting~\cite{ruschendorf1995convergence}. Hence, we note that the agent population mimics the distribution of New York City, but is not an exact twin (since individual-level microscopic signal is not available).

\textbf{Behavior}: When sampling agent behavior using an LLM, we use GPT-3.5 for all our experiments. The user prompts are given in the main paper. The system prompt is provided below:
\begin{tcolorbox}[colback=blue!5!white, colframe=blue!75!black, title=System Prompt]
There is a novel disease. It spreads through contact. It is more dangerous to older people.
People have the option to isolate at home or continue their usual recreational activities outside.
Given this scenario, you must estimate your actions based on
    1) the information you are given,
    2) what you know about the general population with these attributes.

"There isn't enough information" and "It is unclear" are not acceptable answers.
Give a "Yes" or "No" answer, followed by a period. Give one sentence explaining your choice. 
\end{tcolorbox}
We observed marginal behavioral improvements with GPT-4 but did not run scale experiments due to practical considerations (the goal of the paper is to demonstrate capabilities of the framework). We note that AgentTorch API is generic and can integrate with arbitrary offline or online LLM for sampling of behavior.

\text{Environment}: Our experiments focus on the dynamics of disease spread and labor market. We use standard disease~\cite{hinchOpenABMCovid19AgentbasedModel2021b, chopraDifferentiableAgentbasedEpidemiology2023c} and labor models~\cite{li2023large} which have been used extensively in prior work. The disease model capture agent's probability of infection given interaction neighborhood, virus transmissibility ($R_0$) and demographic-specific susceptibility. For disease progression, we follow a standard SEIRM model~\cite{chopraDifferentiableAgentbasedEpidemiology2023c} with discrete transitions at each agent, with generation times obtained from CDC for the delta wave (in progress during December 2020 to April 2021). The labor model captures the unemployment rate based on their individual willingness to work and insured unemployment rates. To make the environment realistic, we capture additional clinical, behavioral and financial interventions - consistent with the protocols in place at that time in the world. First, \underline{Vaccination}: agent's receive vaccines under a two dose vaccination protocol, with 21 days delay by default. We consider behavioral stochasticity where agents may choose to not return for the second dose. Second, \underline{Testing}: agent's have options to receive Antigen or PCR-tests (with their calibrate specificity and result time obtained from CDC data) when they exhibit symptoms. Third, \underline{Stimulus}: Eligible agents receive stimulus payments at specific time intervals, as was implemented in NYC at the time. Specifically, December 2020 - March 2021 overlaps with the second stimulus check which provided adults \$ 600 and additional \$ 600 for every child. We note that AgentTorch helps differentiate through these stochastic dynamics and also scale the environment to large populations (8.4 million agents). Finally, we note while these experiments focused on mechanistic dynamics, the differentiability of AgentTorch allows to specify arbitrary complex dynamics. In other examples, we have modeled simulation environments with convolutional neural networks (on GitHub, see models/nca) or even generative models like LLMs. The code for this environment is available on Github at \href{https://github.com/AgentTorch/AgentTorch/tree/master/models/covid}{models/covid}.

\section{Appendix C: Benchmarking LLM as ABM Agents}
Results in \autoref{sec:benchmark_llm_agents} demonstrated the ability of LLMs to recreate labor force participation behavior across different boroughs on NYC around the time of the second stimulus payment. (December 2020 - March 2021). Here, we provide additional details regarding the ability to recreate similar behavior at different points in time. We consider another time-horizon later in the pandemic (October 2021 - December 2021) when stimulus payments got exhausted. We updated the prompt to include the following: \textit{"it has been number of \{weeks\} since start of the epidemic"}, where \{weeks\} specifies the duration since August 2020.  We observe the response of LLM Archetype and capture it as the monthly percent change in labor force. Result in ~\autoref{fig:appC-fatigue} shows that the predicted labor force behavior exhibits a good correlation with the observed data, across boroughs. To further validate the LLM archetype's behavior, we poll the agents to sample the rationale behind their decisions. We observe agent's routinely mention "pandemic fatigue" which is consistent with real-world discourse from the time. \textit{Interestingly, we observe that different agent interpret this dynamic in different ways with some agents keen to return to work to mitigate financial constraints while other agent's feel depressed and less motivated to go back to work}. We present a few samples of their reasoning below:

\begin{figure}[h!]
    \centering
    \includegraphics[width=0.65\linewidth]{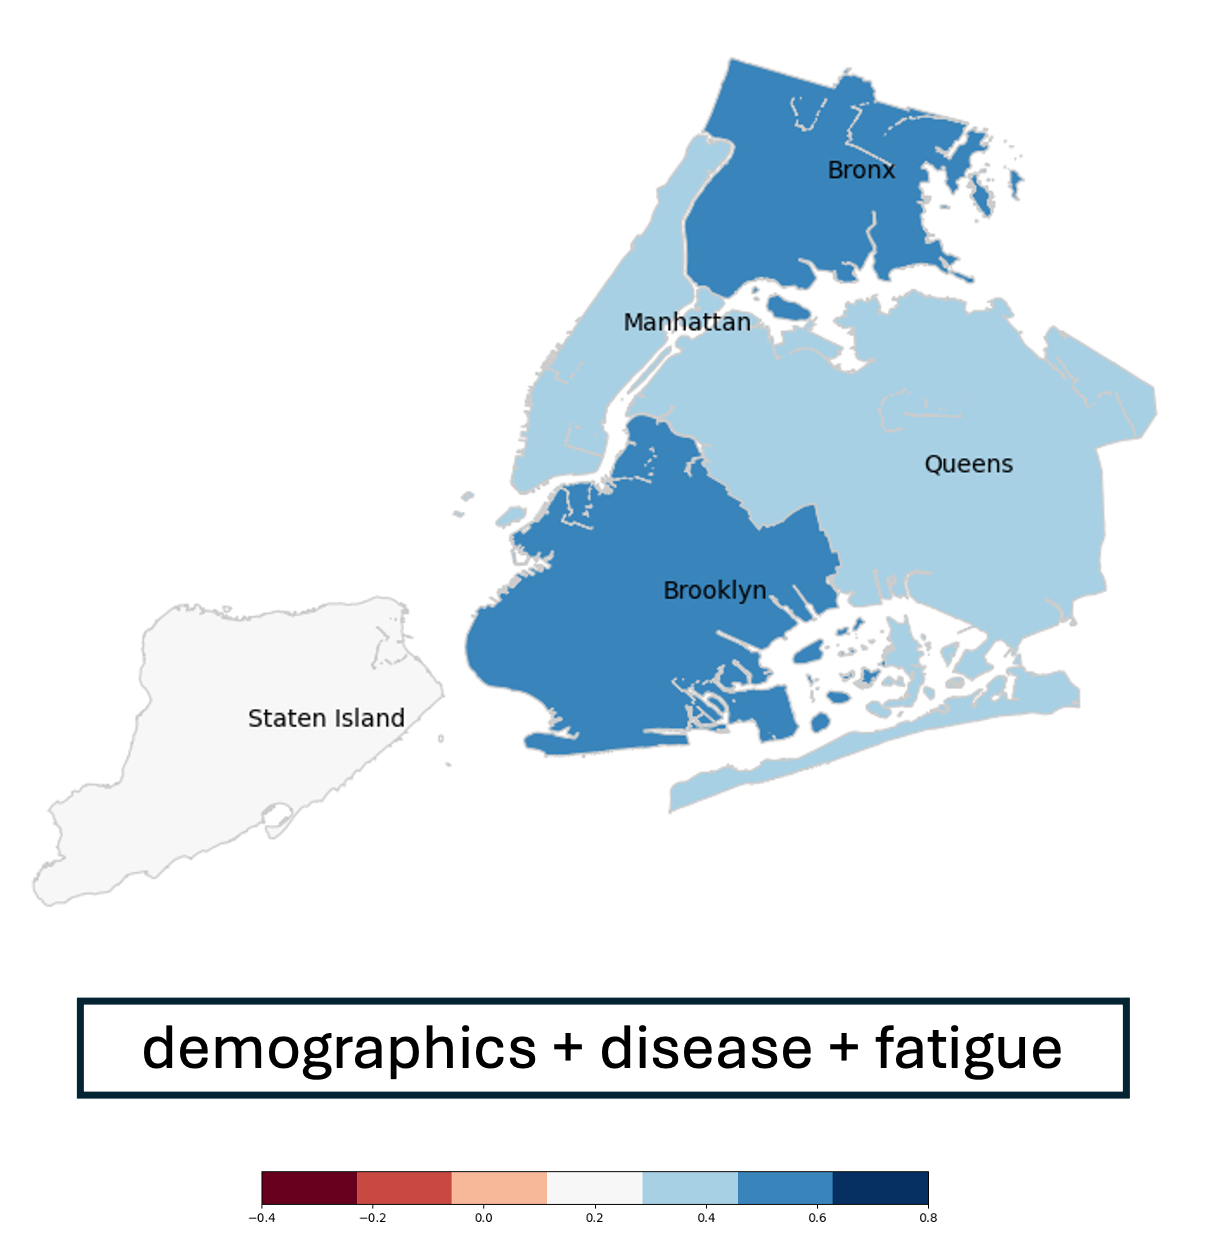}
    \caption{Correlation between estimated and real-world employment participation behavior from \textbf{October 2021 to December 2021}. We consider a later phase in the pandemic (once stimulus payments and unemployment assistance has been discontinued). Here, we capture the labor force behaviour predicted by LLM archetypes in response to pandemic fatigue, and correlate it with the observed data in NYC.}
    \label{fig:appC-fatigue}
\end{figure}

Reasoning 1: \textit{Let's think step by step in order to We have been consistently seeing a low willingness to work of 0.1 over the past few months, indicating a strong impact of pandemic fatigue. Considering the number of COVID cases and it has been 18 months since COVID started, there might be a slight increase in willingness to work due to \textbf{potential financial constraints and fatigue from staying at home for an extended period}.}

Reasoning 2: \textit{Let's think step by step in order to produce the answer. We have been tracking the individual's willingness to work over the past few months, and we can see a gradual increase in their willingness as the number of COVID cases fluctuates. \textbf{Additionally, as time passes, pandemic fatigue may be setting in, leading to a higher willingness to work.} Considering the current number of COVID cases in NYC, and it has been 18 months since COVID started, we can expect the individual's willingness to work to be higher than before.}

Reasoning 3: \textit{Let's think step by step in order to produce the answer. We have been observing a consistent willingness to work of 0.1 over the past few months, \textbf{indicating a very low motivation to work}. Considering the number of COVID cases in NYC is still relatively high and it has been 18 months since the pandemic started, the pandemic fatigue might have increased. This could further decrease the willingness to work.}

We observe similar effects regarding impact of fatigue on isolation behavior, which is discussed in appendix E, below.

\section{Appendix D: Simulating with LLM as ABM agent}
LLMs can capture adaptive agent behavior but are computationally expensive which prohibits simulating large populations. \autoref{sec:calibration} explore the use of LLMs as agents in ABMs, specifically focusing on the this trade-off between agency and simulation scale. Here, we provide details about prompt specification (when LLMs as used as ABM agents) and the setup for the calibration experiment presented in paper

\textbf{Prompt Specification}: The user prompt includes details about individual demographics, time-varying infection statistics, pandemic duration and external interventions. When LLM are used as ABM agents, the prompt inputs are bootstrapped from the simulation. Specifically, we use the case statistics and pandemic duration from the simulation trajectory, instead of ground-truth data. We conduct such "auto-regressive prompting" for two reasons: i) when simulating for prospective interventions, ground-truth data is not available and hence prompt needs to be specified entirely using simulation; ii) when simulation is un-calibrated, the model peaks may not align well with real-world data. In such case, using ground-truth data is unsuitable for capturing the adaptability of behavior (especially when using time-varying information like infections). Hence, since prompt at step $t$ depends upon simulated trajectory at step $t-1$, LLMs need to be sampled online during the simulation. Since behaviors cannot be sampled offline, the trade-off between simulation scale and agent behavior becomes particularly critical. We explored that with the calibration experiment.

\textbf{Calibration Experiment}: 
We compared three agent configurations:
\begin{itemize}
    \item Heuristic: 8.4 million agents with behavior sampled randomly (follows from~\cite{chopraDifferentiableAgentbasedEpidemiology2023c}). This prioritizes simulation scale over agency.
    \item Archetype: 8.4 million agents with 100 LLMs as archetypes. This provides a trade-off between simulation scale and agency.
    \item LLM-Agent: 100 agents with 100 LLMs AS unique per agent (follows from~\cite{parkGenerativeAgentsInteractive2023}). This prioritizes agency over simulation.
\end{itemize}
Archetype samples behavior for each agent based on the variables in the prompt (each simulation agent maps to population archetype). LLM-Agent sub-samples the population, and also re-scales the simulation outputs during calibration.

We conduct calibration with the protocol introduced in~\cite{chopraDifferentiableAgentbasedEpidemiology2023c,quera-bofarullBayesianCalibrationDifferentiable2023,chopra2024framework} where a calibration network (CalibNN) is used to structural parameters and is optimized with gradient from the simulation output. CalibNN is used to predict R0 and IUR for the disease and labor dynamics, respectively and is a GRU (since these parameters are time-varying), as in~\cite{chopraDifferentiableAgentbasedEpidemiology2023c}. Each simulation step is a day for disease dynamics and a month for labor dynamics, consistent with real-world considerations in epidemiology and macroeconomics. For disease model, we aggregate the infection data per week and care with a running average of the CDC case data. For labor model, we compare the unemployment rate estimated at each step with the month-over-month data released by Bureau of labor statistics. We use the MSELoss in both cases. 

CalibNN uses multi-modal context data to estimate the structural parameters. This includes the following signals:
\begin{itemize}
    \item Data signals 1: Mobility signals. The signals originate from the record of people visiting points of interest (POIs) in various regions. According to Google, daily changes in visits to various POI categories are collected and compared with the period January 3-February 6, 2020. Additionally, we collected a daily change of visitors from Apple, which shows the relative volume of directions requested across different US states compared to January 13. Different non-pharmaceutical interventions (NPIs) and different policies adopted by different states are implicitly illustrated by mobility signals.
    \item Data signals 2: Symptomatic surveys. During the pandemic, Facebook collected statistics on COVID-like illness (CLI\%) across the US and different states. On the basis of symptoms reported in voluntary surveys, they estimate this percentage.
    \item Data signals 3: Symptom search data. Google collects records of searches related to symptoms for multiple conditions and syndromes across the US and different states. Their system provides a metric that quantifies search volume associated with specific symptoms, which undergoes a privacy-protecting mechanism before being publicized. We consider the following 14 symptoms: Fever, Low-grade fever, Cough, Sore throat, Headache, Fatigue, Vomiting, Diarrhea, Shortness of breath, Chest pain, Dizziness, Confusion, Generalized tonic–clonic seizure, and Weakness.
    \item Data signals 4: Number of hospitalizations. The US Department of Health \& Human Services provides daily hospitalization admissions dating back to January 1, 2020. Several primary sources provide facility-level granularity reports to create this signal: (1) HHS TeleTracking, (2) reporting provided to HHS Protect by state/territorial health departments on behalf of their healthcare facilities, and (3) the National Healthcare Safety Network.
    \item Data signals 5: Number of new deaths. The Johns Hopkins University reports daily mortality for COVID-19. They collect and curate data from official websites of state public health departments across the US. This has been the source of data for the CDC COVID-19 forecasting initiative.
\end{itemize}

Finally, we hyperparameters use a learning rate of $10^{-4}$, the Adam Optimizer. The initial infections percentage is the percentage of the population that is infected at time step $t=0$ of the simulation; and is initialized with real-world data. All experiments are conducted on a V100 with 32 GB memory. The code is publically available on the github at \href{https://github.com/AgentTorch/AgentTorch/tree/master/models/covid/calibration}{models/covid/calibration}.

\section{Appendix E: Analysis results}

AgentTorch provides the `agent\_torch.Analysis` API to conduct analyses and interventions upon the trace of a simulation. A corresponding code snippet is provided in the main paper (~\autoref{fig:code-analysis}) and a demo video of these capabilities is also included in the README.md for \url{github.com/AgentTorch/AgentTorch}. \url{https://agenttorch.github.io/AgentTorch/tutorials/using-models/} includes a hands-on tutorial to use the analysis capabilities of AgentTorch. We initialize an analyzer as `sim\_analyzer = agent\_torch.Analysis(simulation)`.

\textbf{Retrospective Analysis}: Beyond the results presented in the main paper, `sim\_analyzer.poll` can also be used to query the state of the simulation. A sample snippet is given in the callout below:

\begin{tcolorbox}[colback=blue!5!white, colframe=blue!75!black, title= Example Analysis Query]
sim\_analyzer.poll("Which age group has lowest median income, how much is it?")
\\
\\
Trace - \textit{Invoking: run\_analysis\_on\_simulation\_state with {'query': 'Which age group has the lowest median income and how much is it?'}}
\\
\\
Result - \textbf{The age group with the lowest median income is 20t29 with a median income of \$168.}

\end{tcolorbox}

\textbf{Counterfactual Analysis}: `sim\_analyzer.query` can be used to update subset of the simulation trace and compare the relative impact of this change. We can then use this to ask "what-if" questions. Here, we use this API to analyze the relative impact of behavior change and variant transmissibility on prompt adaption during different stages of the pandemic. Delta ($R_0=[2.5-4.0]$) and Omicron ($R_0=[5.5-8.0]$) were two variants of the COVID-19 pandemic, which emerged at different times. While Omicron was roughly 2-3 times more transmissible that Delta, it produced over 5-20 times the case intensity. This was due to coupled dynamics of behavior and disease. To analyze this, we consider two questions: "what if we had the delta wave later?" and "what if we had the omicron wave earlier?"

\begin{figure}[h!]
    \centering
    \includegraphics[width=0.95\textwidth]{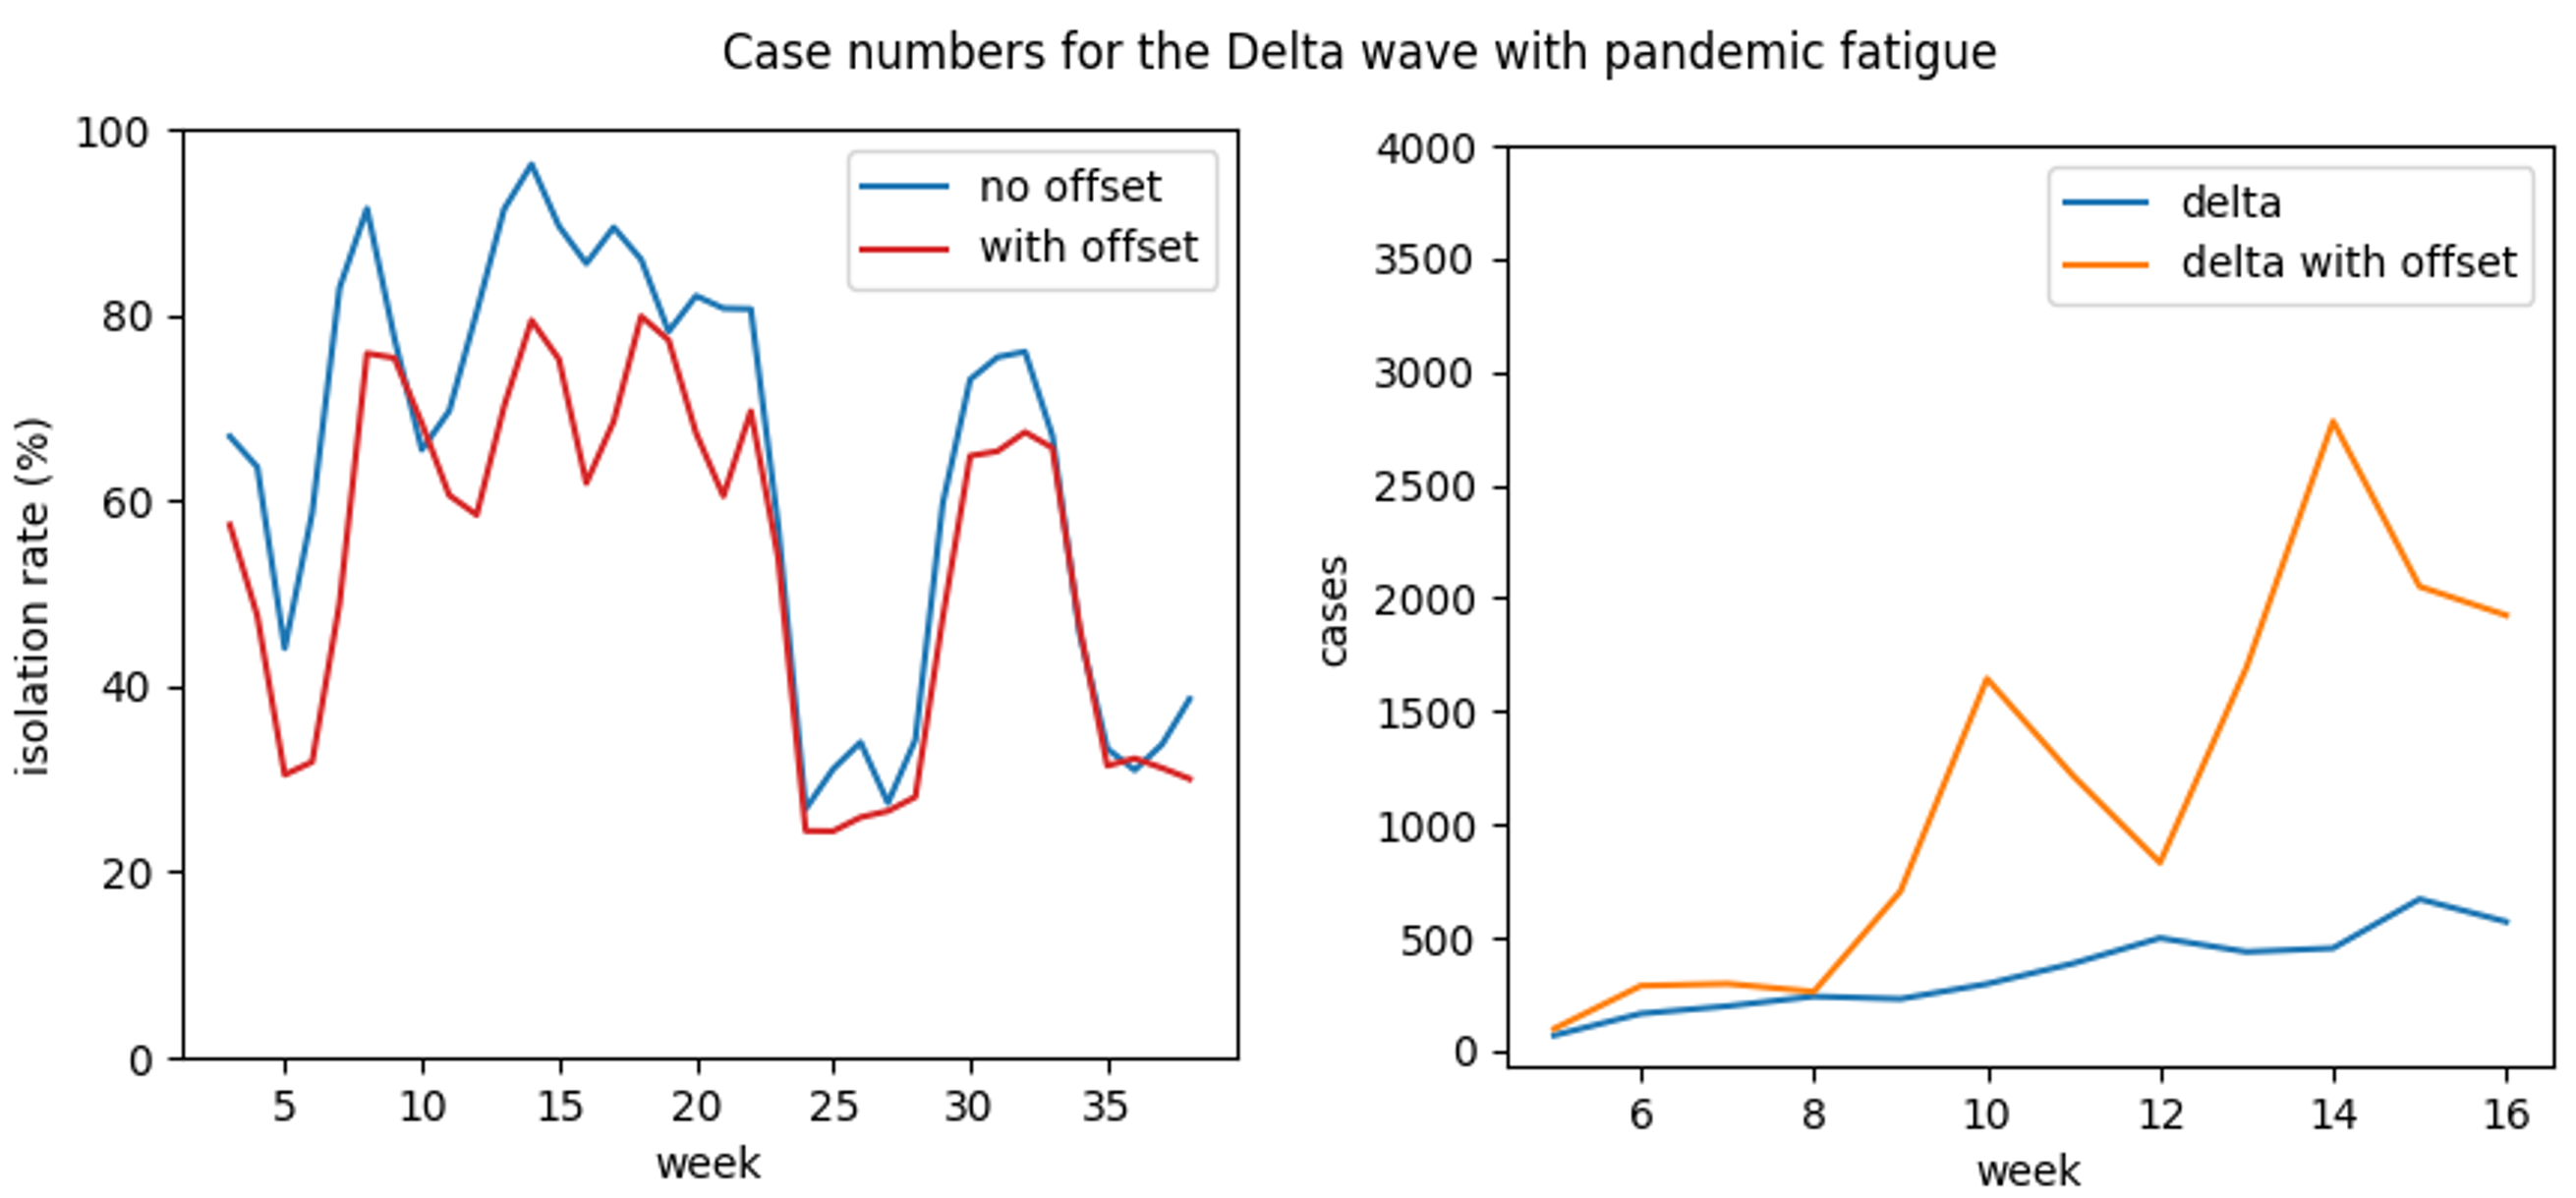}
    \caption{Delayed onset of the delta wave would have been relatively more destructive for the population, due to behavior adaptation. (left) Introducing pandemic fatigue ("the offset") to the prompt reduces relative rates of isolation behavior in the population. (right) This decrease in isolation behavior translates to increased disease transmission in the population.}
    \label{fig:q1-counter}
\end{figure}

\textit{Q1: What if we had the delta wave later?}: The prompt includes details about the duration of the pandemic, \textit{"it has been number of \{weeks\} since start of the epidemic"}. To analyze the effect of time-delay induced behavior change, we update this prompt with an artificial offset in the number of weeks. Then, the prompt looks like this: \textit{"it has been number of \{weeks + ARTIFICIAL-OFFSET \} since start of the epidemic"}. Executing this experiment in straightforward in AgentTorch, with few commands with the analyzer: i) `simulation.update(NEW\_PROMPT)`; iii) `sim\_analyzer.query("how does duration of the pandemic impact disease spread?")`. Results are included in ~\autoref{fig:q1-counter} show that "pandemic fatigue" reduces relative isolation behavior of individuals which results in increased spread of the disease, even for the same transmissible variant. This is evident by the higher peaks observed due to behavior change.

\textit{Q2: What if we had the omicron wave earlier?}: We take our model calibrated to the delta variant and update the $R_0$ in the simulation trace to mimic the omicron variant. We model the effect of the higher transmissible variant, while keeping the same behavioral dynamics in the simulation. The corresponding code snippet is included in ~\autoref{fig:code-analysis} in the main paper. Specifically, we execute the commands: `simulation.update("R0", 5.5)` and `sim\_analyzer.query("how has higher R0 affected infections?")`. Results are included in ~\autoref{fig:q2-counter} help decouple the impact of behavior change and viral transmissibility on producing a disease wave during the pandemic.

\begin{figure}[h!]
    \centering
    \includegraphics[width=0.95\textwidth]{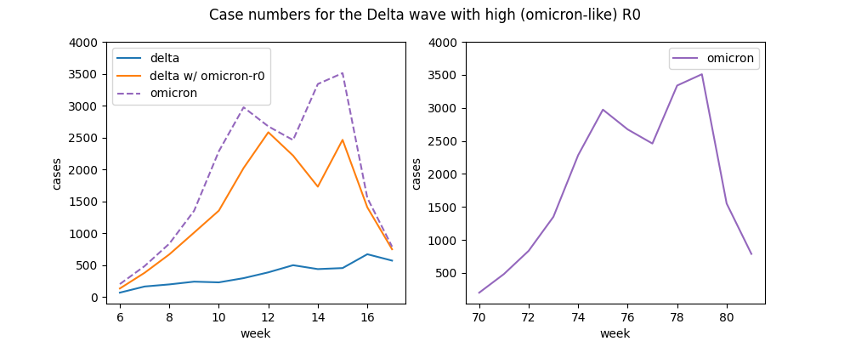}
    \caption{An early onset of "omicron-like variant" would have been more destructive due to more higher transmissibility, but not as much as the eventual omicron wave which also had a coupled influence of the behavior change (additional "pandemic fatigue" due to more time). (left) Comparing the original delta wave (in \textcolor{blue}{blue}), delta wave with "omicron-like" transmissibility (in \textcolor{orange}{orange}) and the omicron wave (shown in \textcolor{mypurple}{dashed purple} since it emerges at a later time) (right) The omicron wave when it emerged later in time (in \textcolor{mypurple}{purple}) achieves a higher peak than both the original and "omicron-like" delta wave due to impact of variant transmissibility and behavior adaptation}
    \label{fig:q2-counter}
\end{figure}

\textbf{Prospective Interventions}: We can use a calibrated model to design interventions for the future, using the `sim\_analyzer.speculate` API. Here, we evaluate the design immunization protocols due the COVID-19 pandemic. In NYC, we followed a two dose vaccination protocol with second dose schedule 3 weeks after the first dose. Due to supply chain constraints and economic constraints, it was required to delay the second dose to mitigate the shortfall. We can use AgentTorch to automatically analyze this design choice. When posed with the question: "What if we delay the second vaccine dose by 2 months?", `sim\_analyzer.speculate` can generates a sequence of hypothesis and execute experiments to measure the sensitivity of the decision. For instance, this decision is sensitive to protection offered by the first dose and immune decay, which was not very well understood at the time (March 2021). The goal is to compare two protocols: a) P1: with standard dosage and b) P2: with delayed second dose. Specifically, AgentTorch generates multiple configurations with different first dose efficacy, runs the two protocols for each configuration; and measure the relative fitness. We define the fitness function as the ratio of simulated deaths in P2 and P1. Delaying the second dose is effective when the fitness is < 1. Results in~\autoref{fig:appE-prospective} show that this can help identify the range when delaying the second dose is a viable strategy.

\begin{figure}
    \centering
    \includegraphics[width=0.72 \textwidth]{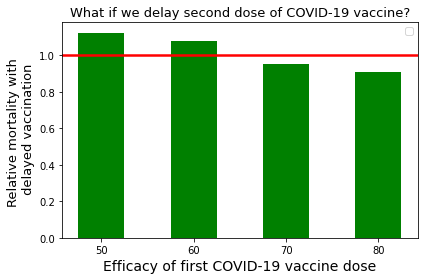}
    \caption{The decision to delay the second dose of the COVID vaccine is sensitive to efficacy of the first dose. AgentTorch allows us to automatically conduct such a sensitivity analysis and measure the viability of a delayed immunization protocol. This protocol is viable if effectiveness of the first dose is above 80\%, which is consistent with real world outcome (single Pfizer vaccine efficacy was 87\%).}
    \label{fig:appE-prospective}
\end{figure}
